# Supplementary material for: Simultaneous reconstruction of evolutionary history and epidemiological dynamics from viral sequences with the birth-death SIR model
Source: arXiv:1308.5140 source file (2014-03-21)
Supplement: Supplementary file 1 [file bdsir_SI.pdf]

# Supplementary information: Simultaneous reconstruction of evolutionary history and epidemiological dynamics from viral sequences with the birth-death $SIR$ model

**Denise Kühnert[1,2], Tanja Stadler[2], Timothy G Vaughan[3,4], Alexei J Drummond[3,5]**

[1]*Department of Environmental Systems Science, ETH Zürich, Switzerland;* [2]*Department of Biosystems Science & Engineering, ETH Zürich, Basel, Switzerland;* [3]*Department of Computer Science,University of Auckland, Auckland, NZ;* [4]*Institute of Veterinary, Animal & Biomedical Sciences, Massey University, Palmerston North, NZ and* [5]*Allan Wilson Centre for Molecular Ecology and Evolution, University of Auckland, Auckland, NZ*

## S1 The probability density of a tree under the BDSIR model

The probability density of a sampled tree under the BDSIR model is given by

$$\begin{aligned}\hat{f}(\mathcal{T}|\{\lambda_i = \beta n_S(i)|i = 0\dots m\}, \mu, \psi, n_S(0), T) &= \frac{q_1(0)}{1-p_1(0)} \prod_{i=1}^{\hat{n}-1} \beta n_S(l(x_i)) q_{l(x_i)}(x_i) \\ &\cdot \prod_{i=1}^{\hat{n}} \frac{\psi}{q_{l(y_i)}(y_i)} \prod_{i=1}^{m} q_{i+1}(t_i)^{n_i},\end{aligned}$$

with $l(t) = i$ if and only if $t_{i-1} \leq t < t_i$, and with $(t_{i-1} \leq t < t_i,\ i = 1, \dots, m)$, $\hat{n}$ denotes the number of sequentially sampled leaves and $n_i$ is the number of lineages in the tree at time $t_i$. Furthermore,

$$p_i(t) = \frac{\lambda_i + \mu + \psi - A_i \frac{e^{-A_i(t-t_i)}(1+B_i)-(1-B_i)}{e^{-A_i(t-t_i)}(1+B_i)+(1-B_i)}}{2\lambda_i}$$

and

$$q_i(t) = \frac{4e^{-A_i(t-t_i)}}{(e^{-A_i(t-t_i)}(1+B_i) + (1-B_i))^2},$$

where

$$\begin{aligned}A_i &= \sqrt{(\lambda_i - \mu - \psi)^2 + 4\lambda_i\psi} \\ B_i &= \frac{(1 - 2(1-\rho_i)p_{i+1}(t_i))\lambda_i + \mu + \psi}{A_i}\end{aligned}$$

for $i = 1, \dots, m$ and $p_{m+1}(t_m) := 1$.

## S2 Stochastic integration of $SIR$ trajectories

In this section we focus on efficiently sampling trajectories $f(\tilde{\mathcal{Y}}|\eta)$ under the stochastic $SIR$ model, i.e. sampling $\{n_S(i), n_I(i), n_R(i)|i = 1 \ldots m\}$, by recording compartment population sizes of the continuous-time model at the discrete times $t_1, \ldots, t_m$. The $SIR$ model is a birth-death process. Birth-death processes are usually expressed in terms of their dynamical effect on a probability distribution over compartment population sizes (i.e. the trajectories). Direct treatment—either analytical or numerical—of the *master equation* [1] is often impossible in all but the very simplest models. A popular alternative, therefore, is to employ the stochastic simulation algorithm (SSA) developed by Gillespie [2, 3]. This algorithm draws samples from the probability distribution over possible trajectories compatible with the model, by directly simulating the random birth-death events which make up the process.

Unfortunately, when applied to $SIR$-type models, the SSA can become numerically inefficient due to the large number of infection and recovery events which can occur, even when the compartment population sizes are reasonably modest. For this reason, we turn instead to the so-called $\tau$-leaping family of algorithms also proposed initially by Gillespie [4]. Such algorithms divide the simulation period into a large number of short time intervals and draw the total number of each type of event expected to occur in each of these intervals from Poissonian distributions. This is analogous to the way in which the numerical integration of differential equations usually proceeds, and it has been shown [5] that Gillespie's $\tau$-leaping is in fact the birth-death process equivalent of an integration algorithm used to numerically solve stochastic differential equations.

In the BDSIR method, we employ the "Step Anticipation $\tau$-Leaping" (SAL) algorithm [6]. This is a more sophisticated method than the original $\tau$-leaping algorithm in that it employs second order corrections to the rates of the Poissonian distributions used to generate the number of events in a given integral. This markedly improves the accuracy that SAL can achieve for a given time interval.

Figure 1 demonstrates the effectiveness of the chosen integration algorithm applied to the stochastic $SIR$ model. Firstly, Fig. 1a compares the expected population sizes within the susceptible, infected and removed compartments calculated using $10^4$ SSA trajectories with those calculated using SAL and an integration time step length of 2 days. (The model parameters used were $\beta = 8.14 \times 10^{-6}$ and $\gamma = 1.362 \times 10^{-3}$, with $n_S(0) = 10^3$ and $n_I(0) = 1$.) The results agree to within the standard error associated with the means (which itself is always non-zero when expectation values are estimated from

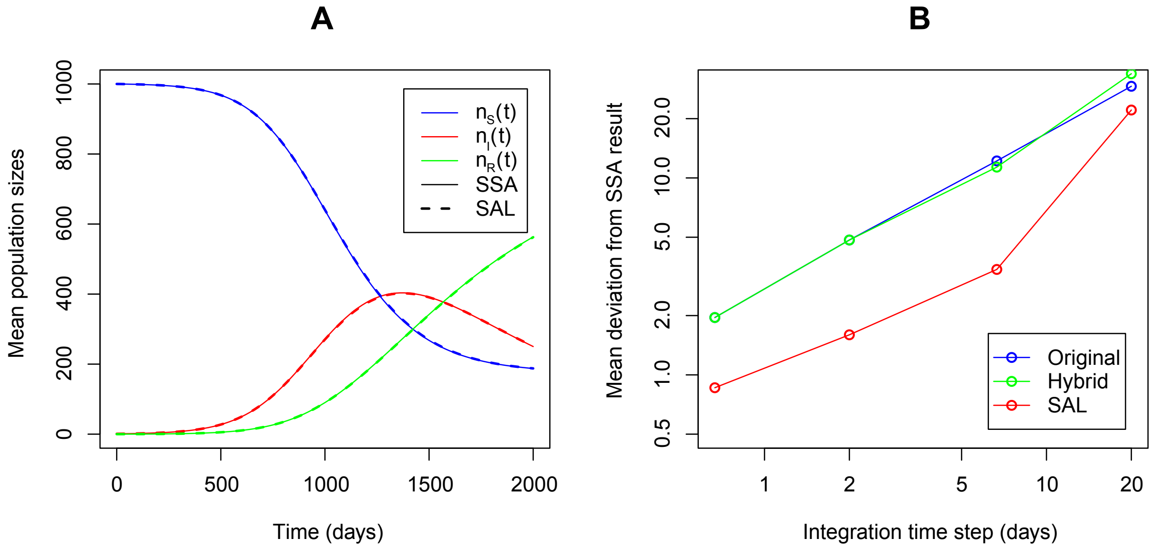


**Figure 1. Validation of the choice of SAL for generation of stochastic SIR trajectories by comparing SAL to the exact, but slow SSA**. (a) Comparison of mean compartment population sizes calculated using $10^4$ SSA trajectories with those calculated using $10^4$ SAL trajectories and a step size of $\tau = 2$ days and model parameters $\beta = 8.14 \times 10^{-6}$, $\gamma = 1.362 \times 10^{-3}$. (b) Time-averaged difference between SSA results for average infected population and results obtained from three different $\tau$-leaping strategies, for four distinct values of $\tau$.

a finite number of trajectories), thus supporting our use of the SAL algorithm as an efficient alternative to the SSA.

Secondly, Fig. 1b illustrates the convergence behaviour of SAL, compared with two other varieties: the original $\tau$-leaping algorithm and the hybrid $\tau$-leaping/SSA algorithm developed by Cao et al. [7]. Error estimates were obtained by calculating the time-averaged difference between the mean infected population sizes obtained from $10^4$ trajectories generated using the $\tau$-leaping method in question and those obtained from $10^4$ SSA trajectories. These results clearly demonstrate the superiority of the SAL algorithm for a given step size over both the original and hybrid $\tau$-leaping schemes, thus validating our choice in using it in the BDSIR method (see below).

In the context of the BDSIR method, we use $10^4$ time steps which we find gives good convergence when compared to the results of Gillespie's direct method.

## BDSIR simulation results with fixed sampling proportion $s$

In this additional set of simulations the sampling proportion $s$ is fixed to the true value. This results in narrower HPD intervals with accurate estimates of $R_0$, $\gamma$ and $n_S(0)$ (SI Tables 1-4, compared to Tables 1-4 in main text).

**Table 1. BDSIR simulation results ($n_S(0)$ fixed)**

| | truth | median | error | bias | relative HPD width | 95% HPD accuracy (%) |
|---|---|---|---|---|---|---|
| $\mathcal{R}_0$ | 2.50 | 2.48 | 0.10 | -0.01 | 0.44 | 94.00 |
| $\gamma$ | 0.30 | 0.30 | 0.10 | 0.02 | 0.51 | 98.00 |

Posterior parameter estimates and accuracy obtained from 100 simulated trees with 100 tips sampled sequentially through time. $n_S(0)$ and $s$ are fixed to the true simulation value. For each parameter, the median over the 100 medians / errors / biases / HPD widths / HPD accuracies is provided.

**Table 2. BDSIR simulation results ($n_S(0)$ fixed)**

| | truth | median | error | bias | relative HPD width | 95% HPD accuracy (%) |
|---|---|---|---|---|---|---|
| $\overline{\mathcal{R}}_1$ | 2.49 | 2.46 | 0.10 | -0.01 | 0.44 | 94.00 |
| $\overline{\mathcal{R}}_2$ | 2.48 | 2.44 | 0.10 | -0.00 | 0.44 | 94.00 |
| $\overline{\mathcal{R}}_3$ | 2.45 | 2.40 | 0.10 | 0.01 | 0.44 | 94.00 |
| $\overline{\mathcal{R}}_4$ | 2.39 | 2.32 | 0.10 | 0.04 | 0.44 | 92.40 |
| $\overline{\mathcal{R}}_5$ | 2.25 | 2.17 | 0.13 | 0.10 | 0.43 | 89.60 |
| $\overline{\mathcal{R}}_6$ | 2.00 | 1.91 | 0.24 | 0.24 | 0.43 | 86.10 |
| $\overline{\mathcal{R}}_7$ | 1.63 | 1.58 | 0.53 | 0.53 | 0.43 | 81.10 |
| $\overline{\mathcal{R}}_8$ | 1.23 | 1.24 | 1.03 | 1.03 | 0.44 | 76.10 |
| $\overline{\mathcal{R}}_9$ | 0.89 | 0.93 | 1.83 | 1.83 | 0.47 | 69.90 |
| $\overline{\mathcal{R}}_{10}$ | 0.65 | 0.74 | 2.86 | 2.86 | 0.51 | 66.22 |

Computed averages for the effective reproduction number from 100 simulated trees with 100 tips sampled sequentially through time. $n_S(0)$ is fixed to the true simulation value. For each parameter, the median over the 100 medians / errors / biases / HPD widths / HPD accuracies is provided. The averages $\overline{\mathcal{R}}_i$ for $i = 1..10$ were computed from the estimated trajectories, $\mathcal{R}_0$, $\gamma$ and $s$.

**Table 3. BDSIR simulation results ($n_S(0)$ estimated)**

| | truth | median | error | bias | relative HPD width | 95% HPD accuracy (%) |
|---|---|---|---|---|---|---|
| $\mathcal{R}_0$ | 2.50 | 2.54 | 0.10 | 0.02 | 0.47 | 94.00 |
| $\gamma$ | 0.30 | 0.30 | 0.10 | 0.0002 | 0.51 | 99.00 |
| $n_S(0)$ | 999.00 | 2022.55 | 1.02 | 1.02 | 4.92 | 94.00 |

Posterior parameter estimates and accuracy obtained from 100 simulated trees with 100 tips sampled sequentially through time. $s$ is fixed to the true simulation value. For each parameter, the median over the 100 medians / errors / biases / HPD widths / HPD accuracies is provided.

**Table 4. BDSIR simulation results ($n_S(0)$ estimated)**

| | truth | median | error | bias | relative HPD width | 95% HPD accuracy (%) |
|---|---|---|---|---|---|---|
| $\overline{\mathcal{R}}_1$ | 2.49 | 2.51 | 0.10 | 0.01 | 2.08 | 100.00 |
| $\overline{\mathcal{R}}_2$ | 2.48 | 2.49 | 0.11 | 0.02 | 2.08 | 100.00 |
| $\overline{\mathcal{R}}_3$ | 2.45 | 2.46 | 0.11 | 0.03 | 2.08 | 100.00 |
| $\overline{\mathcal{R}}_4$ | 2.39 | 2.40 | 0.12 | 0.06 | 2.08 | 100.00 |
| $\overline{\mathcal{R}}_5$ | 2.25 | 2.23 | 0.15 | 0.12 | 2.07 | 100.00 |
| $\overline{\mathcal{R}}_6$ | 2.00 | 1.97 | 0.27 | 0.26 | 2.07 | 100.00 |
| $\overline{\mathcal{R}}_7$ | 1.63 | 1.63 | 0.56 | 0.56 | 2.10 | 100.00 |
| $\overline{\mathcal{R}}_8$ | 1.23 | 1.25 | 1.06 | 1.06 | 2.15 | 99.50 |
| $\overline{\mathcal{R}}_9$ | 0.89 | 0.93 | 1.88 | 1.88 | 2.26 | 99.00 |
| $\overline{\mathcal{R}}_{10}$ | 0.65 | 0.70 | 2.93 | 2.93 | 2.42 | 99.00 |

Computed averages for the effective reproduction number from 100 simulated trees with 100 tips sampled sequentially through time. $n_S(0)$ is estimated in each analysis. For each parameter, the median over the 100 medians / errors / biases / HPD widths / HPD accuracies is provided. The averages $\overline{\mathcal{R}}_i$ for $i = 1..10$ were computed from the estimated trajectories, $\mathcal{R}_0$, $\gamma$ and $s$.

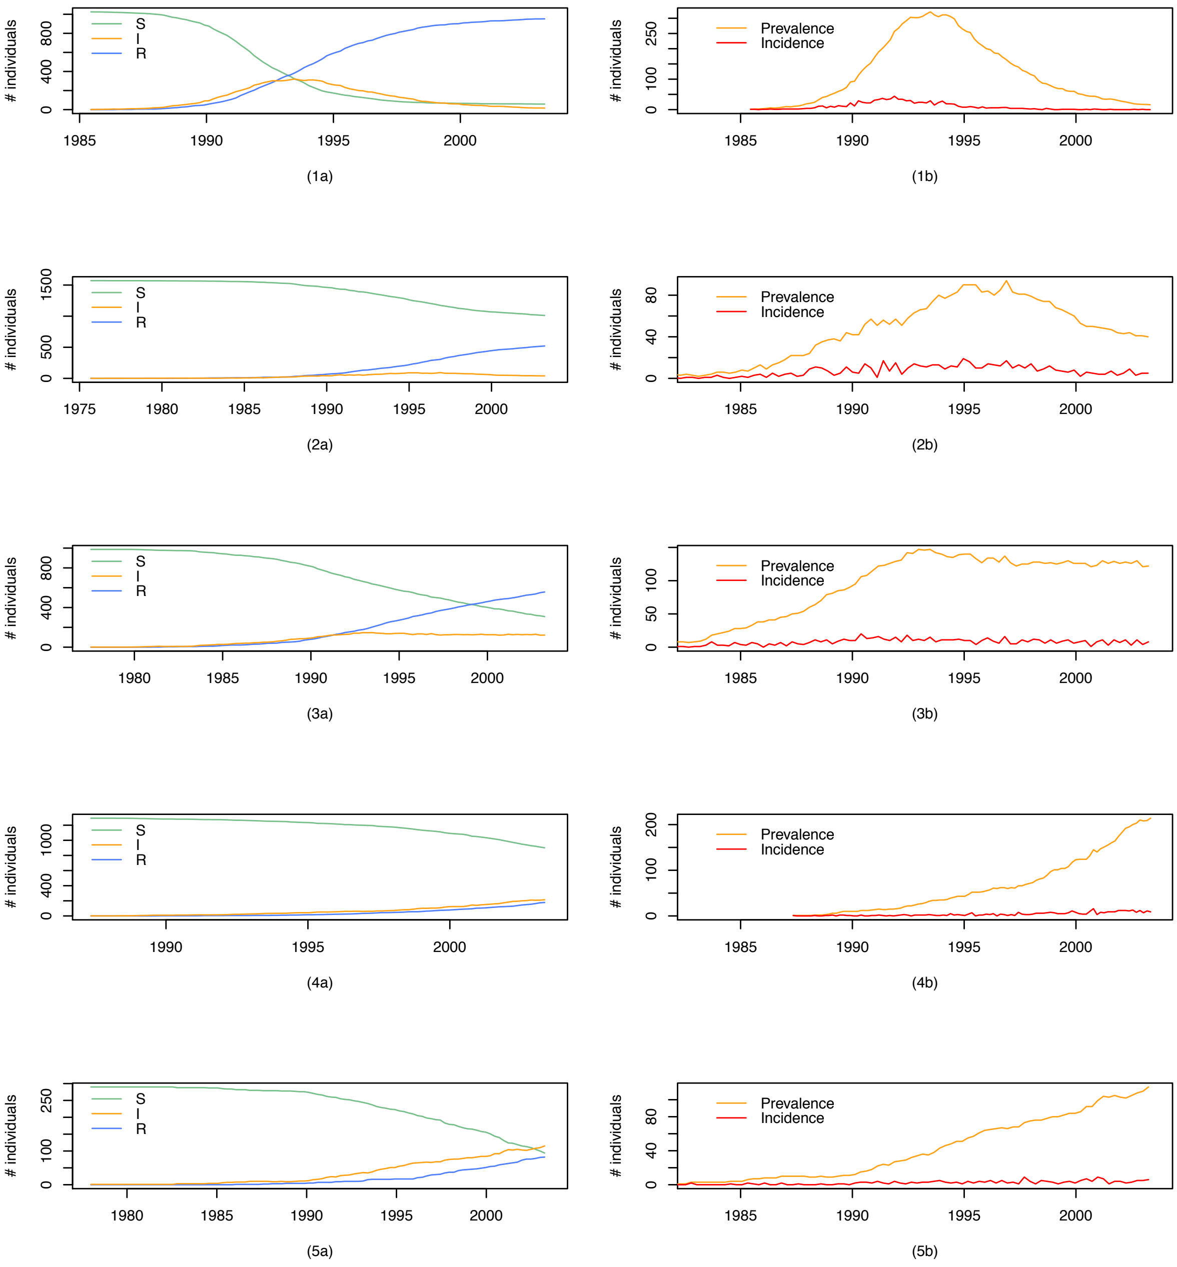


**Figure 2.** $SIR$ **sample trajectories and incidence of HIV-1 clusters from the United Kingdom** A single sample from the trajectory posterior distribution of each cluster (1-5): The overall $SIR$ dynamics (a) show at what stage in the epidemic each cluster was sampled. Zooming into the number of infecteds, i.e. the prevalence over time in (b) enables comparison to the incidence.

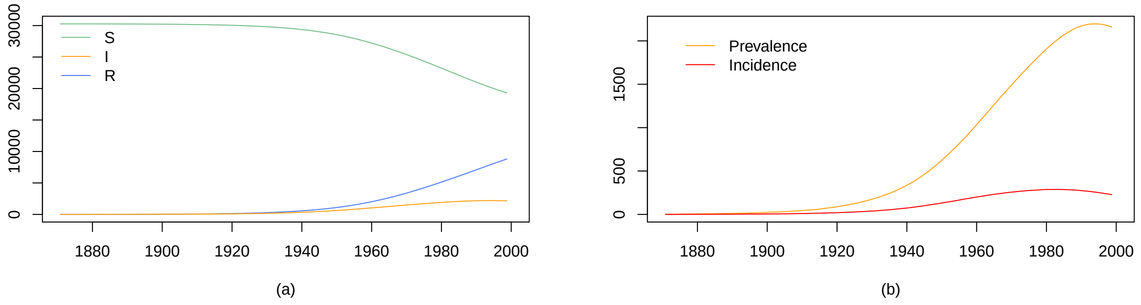


**Figure 3. $SIR$ trajectories and incidence of HCV-2c data from Córdoba province, Argentina** Bayesian posterior median trajectories (a) $SIR$trajectories and (b) incidence and prevalence, estimated under the assumption of small sampling. This analysis resulted in trajectory estimates similar to previous coalescent SIR estimates [8].

# References


[1] van Kampen, N. G. 2007 *Stochastic Processes in Physics and Chemistry.* Elsevier Amsterdam Boston Heidelberg, 3rd edition.

[2] Gillespie, D. T. 1976 A general method for numerically simulating the stochastic time evolution of coupled chemical reactions. *J. Comp. Phys.* **22**, 403.

[3] Gillespie, D. T. 1977 Stochastic simulation of coupled chemical reactions. *J. Phys. Chem.* **81**, 2340.

[4] Gillespie, D. T. 2001 Approximate accelerated stochastic simulation of chemically reacting systems. *J. Chem. Phys.* **115**, 1716. (doi:10.1063/1.1378322).

[5] Li, T. 2007 Analysis of explicit tau-leaping schemes for simulating chemically reacting systems. *Multiscale Modeling and Simulation* **6**, 417. (doi:10.1137/06066792X).

[6] Sehl, M., Alekseyenko, A. V. & Lange, K. L. 2009 Accurate stochastic simulation via the step anticipation tau-leaping (sal) algorithm. *J. Comput. Biol.* **16**, 1195–1208. (doi:10.1089/cmb.2008.0249).

[7] Cao, Y., Gillespie, D. T. & Petzold, L. R. 2005 Avoiding negative populations in explicit poisson tau-leaping. *J Chem Phys* **123**, 054104. (doi:10.1063/1.1992473).

[8] Dearlove, B. & Wilson, D. J. 2013 Coalescent inference for infectious disease: meta-analysis of hepatitis c. *Philos Trans R Soc Lond B Biol Sci* **368**, 20120314. (doi:10.1098/rstb.2012.0314).
